# Supplementary material for: Finding $k$-Secluded Trees Faster
Source: arXiv:2206.09884 source file (2022-06-24)
Supplement: Supplementary file 1 [file appendix.tex]

%\section{Appendix}

% \subsection{Proofs of \cref{sec:subroutines}}
% 
% \begin{lemNoNum}[\cref{lem:safe:contract} restated]
% \lemSafeContract
% \end{lemNoNum}

%\subsection{Proofs of \cref{sec:poc}} \label{ap:poc}

% \begin{lemNoNum}[\cref{lem:combine} restated]
% \lemCombine
% \end{lemNoNum}

% \hui{Before we finish the proof of \cref{lem:algcorrect}, we show the following lemma.}
% \begin{lemma} \label{lem:combine-path}
% Let~$(G,k,F,T,w)$ be an \ELSS{} instance and let~$P$ be a path in~$G$ with~$\degree_G(v) = 2$ for all~$v \in V(P)$ and~$N_G(P) = \{a,b\}$ for some~$a,b \in F$. Let~\kX be a set of descriptions for~$G-V(P)$ such that~$\T_{G-V(P)}(\kX) = \maxset_w(\secl{G-V(P)}{k-1}{F \setminus V(P)})$. Then for all~$p \in V(P) \setminus F$ we have: 
% $$\T_G(\{(r, \X \cup \{\{p\}\}) \mid (r, \X) \in \kX\}) = \maxset_w\{H \in \secl{G}{k}{F} \mid p \in N_G(H)\}.$$
% \end{lemma}
% \begin{proof}
% \hui{
% % First note that~$\{H \in \maxset_w(\secl{G}{k}{F}) \mid p \in N_G(H)\} = \{H \in \maxset_w(\secl{G}{k}{\{a,b\} \cup F}) \mid p \in N_G(H)\}$ since if~$H \in \secl{G}{k}{F}$ with~$\{a,b\} \not\subseteq V(H)$ then~$G[V(H) \cup V(P)]$ is a $k$-secluded tree in~$G$ of larger weight.
% % \bmpr{I don't think this first equality holds. (...) Did you mean: if you take the max-weight supertrees of~$F$, and consider its subset consisting of trees that have~$p$ in the neighborhood, the result is the same as taking the max-weight supertrees of~$\{a,b\} \cup F$ and then take its subset having~$p$ in the neighborhood? Then I think it's true. \hui{Yes, I meant that. I have updated the proof, the lemma statement, its use in \cref{claim:3way:X2}, the statement of \cref{claim:3way:X2} and the two uses of \cref{claim:3way:X2}. \bmp{I think the statement is not correct without additional assumptions; see Slack.}}}
% % In the remainder of the proof we assume that~$\{a,b\} \subseteq F$.
% % \bmpr{Assuming~$\{a,b\} \subseteq F$ is not without loss of generality, as there may not be any max-weight trees in~$G$ containing~$\{a,b\}$. The preceding argument only shows that, in that case, there are no max-weight trees having~$p$ in the neighborhood either.}
% 
% For any~$p \in V(P)$ we define~$\kX^p = \{(r, \X \cup \{\{p\}\}) \mid (r, \X) \in \kX\}$. We show~$\kX^p$ is a valid set of descriptions for~$G$. Note that for any set~$S$ consisting of exactly one vertex from each set~$X \in \X \cup \{\{p\}\}$ there is an~$H \in T_{G-V(P)}(\kX)$ with~$N_G(H) = S\setminus\{p\}$ and~$r \in V(H)$ since~$\kX$ is a valid set of descriptions for~$G-V(P)$. Since~$\{a,b\} \subseteq V(H)$ and~$N_G(P) = \{a,b\}$, we have that~$H' = G[V(H) \cup V(P)]$ is the connected component of~$G-(S \setminus p)$ containing~$r$. Observe that~$H'-p$ is acyclic and connected and since~$p \in V(P) \subseteq V(H')$ we have that~$p \in N_G(H'-p)$, hence~$N_G(H'-p) = S$ and~$\kX^p$ is a valid set of descriptions for~$G$.
% 
% Next we show~$\T_G(\kX^p) \supseteq \maxset_w\{H \in \secl{G}{k}{F} \mid p \in N_G(H)\}$ for any~$p \in V(P) \setminus F$.
% %Consider a maximum weight (with respect to~$w$) $k$-secluded supertree~$H \in \secl{G}{k}{F}$ such that~$p \in N_G(H)$.
% \bmp{Consider a $k$-secluded supertree~$H \in \secl{G}{k}{F}$ which has maximum weight (with respect to~$w$) among those satisfying~$p \in N_G(H)$.}
% We show that~$H \in \T_G(\kX^p)$. By Note~\ref{obs:secluded2} we have that~$H \in \secl{G-p}{k-1}{F}$, that is,~$H$ is a $(k-1)$-secluded supertree of~$F$ in~$G-p$. Observe that~$H-V(P)$ remains connected so~$H-V(P) \in \secl{G-V(P)}{k-1}{F \setminus V(P)}$. We argue that~$H-V(P) \in \maxset_w(\secl{G-V(P)}{k-1}{F \setminus V(P)})$. For the sake of contradiction, suppose there is~$H' \in \maxset_w(\secl{G-V(P)}{k-1}{F \setminus V(P)})$ such that~$w(H') > w(H-V(P))$. Observe that~$H'' := G[V(H') \cup V(P-p)]$ is a connected acyclic subgraph of~$G$ with~$N_G(H'') = N_G(H') \cup \{p\}$, i.e.,~$H''$ is a $k$-secluded supertree of~$F$ in~$G$. Since~$w(H'') = w(H') + w(P-p) > w(H-V(P)) + w(P-p) = w(H)$ this contradicts that~$H \in \maxset_w(\secl{G}{k}{F})$. It follows that~$H-V(P) \in \maxset_w(\secl{G-V(P)}{k-1}{F \setminus V(P)})$. Since it is given that~$\T_{G-V(P)}(\kX) = \maxset_w(\secl{G-V(P)}{k-1}{F \setminus V(P)})$, we have that there is a description~$(r,\X) \in \kX$ for~$G-V(P)$ that describes~$H-V(P)$. Then~$(r, \X \cup \{\{p\}\}) \in \kX^p$ is a description for~$H$ in~$G$ and we conclude that~$H \in \T_G(\kX^p)$ as required.
% 
% Finally we show~$\T_G(\kX^p) \subseteq \maxset_w\{H \in \secl{G}{k}{F} \mid p \in N_G(H)\}$ for any~$p \in V(P) \setminus F$.
% Consider some tree~$J \in \T_G(\kX^p)$. We show that~$J \in \maxset_w \{H \in \secl{G}{k}{F} \mid p \in N_G(H)\}$.
% Clearly~$J \in \{H \in \secl{G}{k}{F} \mid p \in N_G(H)\}$, so it remains to show that~$w(J) \geq w(J')$ for all~$J' \in \{H \in \secl{G}{k}{F} \mid p \in N_G(H)\}$. Suppose for contradiction that there exists such a~$J'$ for which~$w(J) < w(J')$. Observe that~$J - V(P)$ and~$J' - V(P)$ are both $(k-1)$-secluded supertrees of~$F \setminus V(P)$ in~$G-V(P)$, i.e., they are contained in~$\secl{G-V(P)}{k-1}{F \setminus V(P)}$. Since~$V(P-p) \subseteq V(J)$ and~$V(P-p) \subseteq V(J')$ we have that~$w(J-V(P)) < w(J'-V(P))$, so~$J-V(P) \not\in \maxset_w(\secl{G-V(P)}{k-1}{F \setminus V(P)})$. Recall that~$J \in T_G(\kX^p)$ and consider the description~$(r,\X \cup \{\{p\}\}) \in \kX^p$ that describes~$J$. Observe that~$(r,\X)$ describes~$J-V(P)$ in~$G-V(P)$, i.e.,~$J-V(P) \in \T_{G-V(P)}(\kX)$. However it is given that~$\T_{G-V(P)}(\kX) = \maxset_w(\secl{G-V(P)}{k-1}{F \setminus V(P)})$, a contradiction. Hence~$J \in \maxset_w\{H \in \secl{G}{k}{F} \mid p \in N_G(H)\}$.
% }
% \qed
% \end{proof}

% \begin{lemNoNum}[\cref{lem:algcorrect} restated]
% \lemAlgcorrect
% \end{lemNoNum}

%\subsection{Proofs of \cref{sec:time}}
% \hui{Before we prove \cref{lem:NT-large}, we prove two additional lemmas. The first states that under certain conditions, the neighborhood of~$T$ does not decrease during the execution of a single recursive call.} \bmp{In the following, we use the term \emph{leaf} of a (possibly cyclic) graph~$G$ to denote a vertex of degree at most~$1$.}
% 
% \begin{lemma} \label{lem:NT-nondecr}
%  Let~$(G_0,k_0,F_0,T_0,w_0)$ be an \ELSS{} instance such that all leaves of \bmp{$G_0$} are contained in \bmp{$T_0$}. If the algorithm does not terminate before Step~\ref{alg:3way}, then the instance~$(G',k',F',T',w')$ when executing Step~\ref{alg:3way} satisfies~$|N_{G'}(T')| \geq \bmp{|N_{G_0}(T_0)|}$.
%  
%  
%  %Let~$(G,k,F,T,w)$ be an \ELSS{} instance. If the algorithm does not terminate before Step~\ref{alg:3way}, then the instance~$(G',k',F',T',w')$ when executing Step~\ref{alg:3way} satisfies~$|N_{G'}(T')| \geq 1$. If all leaves of~$G$ are contained in~$T$ then~$|N_{G'}(T')| \geq |N_G(T)|$.
% \end{lemma}
% \begin{proof}
% %Since the algorithm does not terminate before Step~\ref{alg:3way} it follows that Steps~\ref{alg:2nbrs} and~\ref{alg:greedy} are not executed, so consider the part of the algorithm before Step~\ref{alg:2nbrs}. By Property~\ref{prop:before-step1} we have hat~$N_{G'}(F') \neq \emptyset$ and~$G'$ is connected. Since~$T'$ is a non-empty connected set\jjhr{maybe add the this is maintained to Property~\ref{prop:before-step1}}, we get that~$|N_{G'}(T')| \geq 1$.
% 
% %For the second statement, suppose
% Since the algorithm does not terminate before Step~\ref{alg:3way} it follows that Steps~\ref{alg:2nbrs} and~\ref{alg:greedy} are not executed, so consider the part of the algorithm before Step~\ref{alg:2nbrs}.
% \bmp{Throughout the proof we use~$(G,k,F,T,w)$ to refer to the instance at the time the algorithm evaluates it; initially~$(G,k,F,T,w) = (G_0,k_0,F_0,T_0,w_0)$, but actions such as contracting leaves may change the instance during the execution}. Suppose that all leaves of~$G$ are contained in~$T$. 
% \bmp{We infer} that~$G[F]$ is acyclic, as otherwise \bmp{the algorithm} would return~$\emptyset$ \bmp{before reaching Step~\ref{alg:3way}}. Removing the connected components of~$G$ that do not contain a vertex of~$F$ does not alter~$|N_G(T)|$. Afterwards we \bmp{know} that~$G$ is connected, as otherwise \bmp{the algorithm} would return~$\emptyset$. Consider a single degree-1 contraction step of a vertex~$v$ with~$F \neq \{v\}$ that results in the instance~$(G-v, k, F^*,T^*, w^*)$. Since we assume that all leaves are contained in~$T$, we have that~$v \in T$. Let~$u$ be the neighbor of~$v$. By Definition~\ref{def:contract} we \bmp{have}~$F^* =  (F \setminus \{v\}) \cup \{u\}$ and~$T^* = (T \setminus \{v\}) \cup \{u\}$. If~$u \in T$, then~$N_{G-v}(T^*) = N_G(T)$ and therefore their size is equal. If~$u \notin T$, then observe that~$u$ cannot be a leaf in~$G$ by assumption and therefore~$N_G(u) \setminus \{v\} \neq \emptyset$. Since~$T$ is connected and~$v$ is a leaf in~$T$ we get~$(N_G(u) \setminus \{v\}) \cap T = \emptyset$. It follows that~$|N_{G-v}(T^*)| \geq |N_G(T)|$. These arguments can be applied for each consecutive contraction step to infer~$|N_G(T)| \geq |N_{G_0}(T_0)|$ \bmp{for the instance~$(G,k,F,T,w)$ after all contractions.}
% 
% Next consider the step where if~$N_G(T)$ contains a vertex~$v \in F$, the vertex~$v$ is added to~$T$. Since~$G[F]$ is acyclic,~$G[T]$ is connected, and~$v \notin T$ is not a leaf, it follows that~$N_G(v) \setminus T \neq \emptyset$ and~$|N_G(v) \cap T| = 1$. It follows that~$|N_G(T \cup \{v\})| \geq \bmp{|N_G(T)|}$. Again these arguments can be applied iteratively. \bmp{For the instance~$(G,k,F,T,w)$ to which this step can no longer be applied,~$G[T]$ is a connected component of~$G[F]$.}
% 
% Next we get that~$N_G(F) \neq \emptyset$ as otherwise the algorithm would return~$\{(r,\emptyset)\}$ for some~$r \in F$. We also get~$k > 0$, as otherwise~$\emptyset$ would have been returned. 
% 
% Since none of the steps decreased the \bmp{size of the} neighborhood of~$T$, \bmp{for the instance~$(G',k',F',T',w')$ at the time Step~\ref{alg:3way} is executed we conclude~$|N_{G'}(T')| \geq |N_{G_0}(T_0)|$ as required.}
% \end{proof}
% 
% \hui{The second lemma required for the proof of \cref{lem:NT-large} states that the \bmp{size of the} neighborhood of~$T$ strictly increases as we make the recursive call in Step~\ref{alg:3way}.}
% 
% \begin{lemma} \label{lem:NT-incr}
% If the instance when executing Step~\ref{alg:3way} is~$(G,k,F,T,w)$ and Step~\ref{alg:3way}(c) branches on the instance~$(G,k,F \cup V(P),T \cup V(P),w)$, then either~$|N_G(T \cup V(P))| > |N_G(T)|$ or some vertex~$u \in N_G(T \cup V(P))$ is adjacent to at least two vertices in~$T \cup V(P)$.
% \end{lemma}
% \begin{proof}
% Consider the path~$P = (v = v_1, \dots, v_\ell)$ with~$\degree_G(v_i) = 2$ for each~$1 \leq i < \ell$ and ($v_\ell \in N_G(T)$ or~$\degree_G(v_\ell) > 2)$ as defined in Step~\ref{alg:3way}. The precondition of Step~\ref{alg:3way}(c) gives that~$G[F \cup V(P)]$ is acyclic. Since~$T \subseteq F$, this implies that~$G[T \cup V(P)]$ is acyclic. It follows that~$V(P) \cap N_G(T) = \{v\}$ and~$\degree_G(v_\ell) > 2$.
% %First suppose that~$u \in N_G(T)$ for some vertex~$u \in N_G(v_\ell) \setminus P$. Then the second condition holds;~$u$ has at least one neighbor in~$T$ as~$u \in N_G(T)$ and~$u$ is adjacent to~$v_\ell \notin T$.
% %Next suppose that~$(N_G(v_\ell) \setminus P) \cap N_G(T) = \emptyset$. Observe that~$N_G(T \cup V(P)) = (N_G(T) \setminus \{v\}) \cup (N_G(v_\ell) \setminus V(P))$. Since~$\degree_G(v_\ell) > 2$ it follows that~$|N_G(T \cup V(P))| > |N_G(T)|$.
% Hence~$|N_G(T) \setminus \{v\}| = |N_G(T)|-1$ and~$|N_G(v_\ell) \setminus V(P)| \geq 2$.
% Observe that~$N_G(T \cup V(P)) = (N_G(T) \setminus \{v\}) \cup (N_G(v_\ell) \setminus V(P))$ so if~$(N_G(T) \setminus \{v\}) \cap (N_G(v_\ell) \setminus V(P)) = \emptyset$ we have~\bmp{$|N_G(T \cup V(P))| > |N_G(T)|$}. Alternatively, suppose~$u \in (N_G(T) \setminus \{v\}) \cap (N_G(v_\ell) \setminus V(P))$. Then the second condition holds;~$u$ has at least one neighbor in~$T$ as~$u \in \bmp{N_G(T) \setminus \{v\}}$ and~$u$ is adjacent to~$v_\ell \notin T \setminus \{v\}$.
% \end{proof}

% \hui{Using \cref{lem:NT-nondecr,lem:NT-incr} we can now prove \cref{lem:NT-large}.}
% \begin{lemNoNum}[\cref{lem:NT-large} restated]
% \lemNTlarge
% \end{lemNoNum}
% 
% We now proceed with the runtime analysis of the algorithm.
% 
% % \begin{lemma} \label{lem:runtime}
% %     The algorithm described in \cref{sec:alg} can be implemented to run in time~$2^{\Oh(k\log k)} \cdot n^3$.
% % \end{lemma}
% \begin{lemNoNum}[\cref{lem:runtime} restated]
%  \lemRuntime
% \end{lemNoNum}

%\subsection{Proofs of~\cref{sec:enum_count}}

% \begin{thmNoNum}[\cref{thm:enumeration} restated]
%  \thmEnumeration
% \end{thmNoNum}
% 
% \begin{thmNoNum}[\cref{thm:counting} restated]
%  \thmCounting
% \end{thmNoNum}

\iffalse
\subsection{Faster Step~\ref{alg:greedy}}

\hui{More efficient algorithm for \cref{lem:greedy:naive}}

\begin{lemma} \label{lem:greedy}
 There is an algorithm that, given an almost leafless \ELSS{} instance~$(G,k,F,T,w)$ such that no vertex in~$N_G(T)$ has more than one neighbor in~$T$, runs in time~$\Oh(n)$ and either
 \begin{enumerate}
  \item returns a vertex~$v$ such that any $k$-secluded supertree~$H$ of~$F$ in~$G$ satisfies~$v \in N_G(H)$, or
  \item concludes that either~$N_G(T) \leq k(k+1)$ or no $k$-secluded supertree of~$F$ exists in~$G$.
 \end{enumerate}
\end{lemma}
\begin{proof}
 Initialize for each vertex in~$v \in V(G)$ a counter~$f(v)$ as follows:
 \begin{align*}
  f(v) = \begin{cases}
          1 &\text{if $v \in N_G(T)$}\\
          0 &\text{otherwise.}
         \end{cases}
 \end{align*}
For each~$v \in N_G(T)$ we execute the following procedure (which may terminate the algorithm by returning a vertex):
\begin{enumerate}
 \item \label{greedyalg:init}
	Intialize~$P_v := (v)$.
 \item \label{greedyalg:extend}
	Let~$y$ be the last vertex of~$P_v$. If~$P_v$ consists of only a single vertex, then let~$x \in T \cap N_G(y)$, otherwise let~$x$ be the second to last vertex of~$P_v$. Take an arbitrary vertex~$z \in N_G(y) \setminus \{x\}$. If~$z \not\in V(P_v)$, append~$z$ to the path~$P_v$ and increase~$f(z)$ by one. Otherwise if~$z \in V(P_v)$, stop this procedure and continue to the next~$v \in N_G(T)$, if any. \huir{counter doesn't work, needs to be like original algorithm}
 \item \label{greedyalg:continue}
	If~$f(z) = 1$ continue extending~$P_v$ by going back to Step~\ref{greedyalg:extend}.
 \item \label{greedyalg:terminate}
	If~$f(z) \geq k+2$ then return~$u'$.
\end{enumerate}
If no vertex has been returned after executing the above procedure for all vertices~$v \in N_G(T)$ then \hui{TODO}

\subsubsection{Runningtime}
Clearly~$f$ can be initialized in~$\Oh(n)$ time. The vertex set~$N_G(T)$ can be determined using DFS starting from a vertex in~$T$. Since~$G[T]$ is acyclic, this takes in~$\Oh(n)$ time. Next, observe that every operation in Steps~\ref{greedyalg:init} to~\ref{greedyalg:terminate} individually can be performed in~$\Oh(1)$ time. In particular, to find a vertex~$z \in N_G(y) \setminus \{x\}$ in Step~\ref{greedyalg:extend} we only need to consider at most two neighbors of~$y$, so this takes~$\Oh(1)$ time. Clearly the proceduce described in Steps~\ref{greedyalg:init} to~\ref{greedyalg:terminate} is executed at most~$|N_G(T)| \in \Oh(n)$ times, so it remains to show that accumulatevely, Step~\ref{greedyalg:extend} is performed only~$\Oh(n)$ times. Note that any time Step~\ref{greedyalg:extend} is performed, the counter~$f(v)$ is increased for some vertex~$v$, and since the procedure stops repeating Step~\ref{greedyalg:extend} once it enounters a vertex whose counter was already incremented before. So all vertices considered in Step~\ref{greedyalg:extend}, except possibly the last, have not been encountered in a previous iteration of Step~\ref{greedyalg:extend}. It follows that the total number of times Step~\ref{greedyalg:extend} is performed is at most~$|V(G)| + |N_G(T)| \in \Oh(n)$ times. Hence the algorithm takes at most~$\Oh(n)$ time.

\subsubsection{Running time}
\begin{claim}
 At any time in the algorithm, there are at least~$f(v)$ distinct paths from~$N_G(T)$ to~$v$ that intersect only in~$v$ and do not contain vertices from~$T$.
\end{claim}
\begin{claimproof}
 \hui{TODO}
\claimqed
\end{claimproof}

\begin{claim}
 If for any vertex~$v \in V(G)\setminus F$ there are~$k+2$ distinct paths from~$N_G(T)$ to~$v$ that intersect only in~$v$ and do not contain vertices from~$T$, then any $k$-secluded supertree~$H$ of~$F$ in~$G$ satisfies~$v \in N_G(H)$.
\end{claim}
\begin{claimproof}
 See \cref{lem:greedy}
\claimqed
\end{claimproof}

\begin{claim}
 If~$G$ contains a $k$-secluded supertree~$H$ of~$F$ and~$N_G(T) > k(k+1)$ then the algorithm returns a vertex.
\end{claim}
\begin{claimproof}
 \hui{TODO}
\end{claimproof}

I think that's it?
\qed
\end{proof}

\hui{Stronger variant (could be used to limit recusion depth to~$\Oh(k^2)$):}
\begin{lemma}
 There is an algorithm that, given an almost leafless \ELSS{} instance~$(G,k,F,T,w)$ such that no vertex in~$N_G(T)$ has more than one neighbor in~$T$, runs in time~$\Oh(n)$ and
 \begin{enumerate}
  \item If~$G$ contains a $k$-secluded supertree of~$F$ and there exists a vertex~$v \in V(G)\setminus F$ with~$k+2$ distinct paths to~$N_G(T)$ that intersect only in~$v$ and do not contain vertices from~$T$, then the algorithm returns such a vertex.
  \item Otherwise it concludes that no $k$-secluded supertree of~$F$ exists in~$G$ or there exists no vertex~$v \in V(G)\setminus F$ with~$k+2$ distinct paths to~$N_G(T)$ that intersect only in~$v$ and do not contain vertices from~$T$.
 \end{enumerate}
\end{lemma}

\begin{lemma}
 If~$(G,k,F,T,w)$ is an \ELSS{} instance and ~$v \in V(G)\setminus F$ is a vertex such that there are~$k+2$ distinct paths from~$N_G(T)$ to~$v$ that intersect only in~$v$ and do not contain vertices from~$T$, then any $k$-secluded supertree~$H$ of~$F$ in~$G$ satisfies~$v \in N_G(H)$.
\end{lemma}
\begin{claimproof}
 See \cref{lem:greedy}
\claimqed
\end{claimproof}

\begin{lemma}
 If~$(G,k,F,T,w)$ is an almost leafless \ELSS{} instance such that~$N_G(T) > k(k+1)$ and~$G$ contains a $k$-secluded supertree of~$F$, then there exists a vertex~$v \in V(G) \setminus F$ such thatthere are~$k+2$ distinct paths from~$N_G(T)$ to~$v$ that intersect only in~$v$ and do not contain vertices from~$T$.
\end{lemma}



\hui{Old:}
\begin{lemma} \label{lem:apply-rule-paths}

 
 If~$(G,k,F,T,w)$ is an MSST instance where~$G$ is connected and has minimum degree 2 and~$G[T]$ has a connected component~$T'$ with~$|N_G(T')| > k(k+1)$, then we can apply one of \cref{rule:2neighbors,rule:loop,rule:paths} in linear time or correctly \hui{abort}.
 %If~$(G,k,T,w)$ is a clean LSST instance and~$|N_G(T)| > k(k+1)$ then we can find a vertex~$v \in V(G) \setminus T$ in linear time such that \cref{rule:paths} applies, or report that~$G$ has no $k$-secluded tree containing~$T$.
 %\hui{Instead of using the concept ``clean'', we could also state that if~$|N_G(T)| > k(k+1)$ then we can apply some reduction rule in linear time.}
\end{lemma}

\begin{proof}
\textbf{Algorithm}
Let~$T'$ be the vertex set of a connected component of~$G[T]$ with~$|N_G(T')| > k(k+1)$. If any of the vertices in~$N_G(T')$ have two or more neighbors in~$T'$ then we can apply \cref{rule:2neighbors}. Otherwise we create a set~$\P$ of~$|N_G(T')|$ paths, each starting from a different vertex in~$v \in N_G(T')$. Initially all paths contain only this vertex. For each path~$P \in \P$, we extend~$P$ in a recursive manner:
\begin{itemize}
 \item If~$P$ contains one vertex~$v$, then~$v \in N_G(T')$. Since~$G$ has minimum degree~2 and \cref{rule:2neighbors} does not apply,~$v$ has at least one neighbor~$u$ not in~$T'$. Append~$u$ to~$P$ as the last vertex.
 
 \item If~$P$ contains more than one vertex, then consider the last and second to last vertices~$v$ and~$v'$ respectively. Since~$v$ has degree at least~2,~$v$ has a neighbor that is not~$v'$. Let~$u$ be such a neighbor.
%    \jjhr{Should~$u$ be disjoint from~$T'$? \hui{Yes, but this never happens: if~$u \in T'$ then there must a vertex earlier in the path that is in~$N_G(T')$, which is a vertex already contained in a path, the path will not be extended further and~$u$ won't be reached. I think the limit on how far a path is extended is only necessary for the running time, for correctness the paths need not be disjoint from~$T'$.}}
 If~$u \not\in P$ then append~$u$ to~$P$ as the last vertex. Otherwise, terminate the recursion.
\end{itemize}
If~$u \not\in P'$ for any~$P' \in \P$ then continue to extend the path recursively. If~$u \in N_G(T')$ and~$\degree_G(p)=2$ for all~$p \in V(P)$ then~$P$ is a $uv$-path for which we can apply \cref{rule:loop}. Otherwise, terminate the recursion.

% Once all paths in~$\P$ have been extended, consider the graph~$G'$ obtained from~$G$ through the following steps:
% \begin{enumerate}
%  \item Remove any edge that is not contained in a path~$P \in \P$ and does not have a vertex from~$T$ as an endpoint.
%  \item Exhaustively remove any vertex of degree less than two that is not contained in~$T$.
% \end{enumerate}
Now let~$G''$ be the graph obtained from~$G$ by removing any edge that is not contained in a path~$P \in \P$ and does not have a vertex from~$T'$ as an endpoint.
Let~$G'$ be the graph obtained from~$G''$ by exhaustively removing any vertex of degree less than two that is not contained in~$T'$.
If there is a vertex~$v \in V(G')\setminus T'$ with~$\degree_{G'}(v) \geq k+2$ then we show there are~$k+2$ distinct paths from~$N_G(T')$ to~$v$ that intersect only in~$v$ and do not contain vertices from~$T'$, hence we can apply \cref{rule:paths}. Otherwise we correctly \hui{abort}.

It is easily verified that this algorithm runs in linear time.

\textbf{Correctness}
We first show that if the algorithm returns a vertex~$v$, then \cref{rule:paths} applies to this vertex. For this consider the graph~$G'$ as obtained in the algorithm.

\begin{claim} \label{claim:paths:forest-and-leaves}
 The graph~$G'-T$ is a forest and all leaves are in~$N_G(T)$.
\end{claim}
\begin{claimproof}
 \hui{TODO}
\end{claimproof}

Clearly if~$v$ has degree at least~$k+2$ in the forest~$G'-T$ then there are~$k+2$ distinct paths from~$v$ to a leaf of~$G'-T$ that intersect only in~$v$. Such a leaf is contained in~$N_G(T)$. Since~$G'-T$ is a subgraph of~$G$ it follows that~$G$ contains~$k+2$ distinct paths from~$v$ to~$N_G(T)$ that intersect only in~$v$, i.e., \cref{rule:paths} applies.
So suppose that~$\degree_{G'-T}(v) \leq k+2$, then since~$\degree_{G'}(v) \geq k+2$ we know that~$N_{G'}(v)$ contains vertices from~$T$, i.e.,~$v \in N_{G'}(T) \subseteq N_G(T)$. Since the instance is clean,~$N_G(v)$ contains at most one vertex from~$T$, so~$\degree_{G'-T}(v) \geq \degree_{G'}(v)-1 \geq k+1$. Then clearly, since~$G'-T$ is a forest, there are at least~$k+1$ paths in~$G'$ from~$v$ to a leaf of~$G'-T$ that intersect only in~$v$. These leaves are all contained in~$N_G(T)$. Since~$v \in N_G(T)$ is not a leaf, the path consisting of only the vertex~$v$ is distinct from the other~$k+1$ paths from~$v$ to~$N_G(T)$. We conclude that~$G$ (which contains~$G'-T$ as subgraph) has at least~$k+2$ distinct paths from~$v$ to~$N_G(T)$ that intersect only in~$v$.

To complete the correctness proof we show that if~$G$ has a $k$-secluded tree~$H$ with~$V(H) \supseteq T$, then~$G'$ contains a vertex~$v \in V(G') \setminus T$ with~$\degree_{G'}(v) \geq k+2$.
Consider the graph~$G''$ obtained in the algorithm, we show that~$G''$ contains a $k$-secluded tree~$H'$ with~$V(H') \subseteq T$. Note that~$G''$ is a subgraph of~$G$ and~$G[T] = G''[T]$ is connected. Let~$H'$ be the connected component of~$G''[V(H)]$ that contains all vertices from~$T$ and observe that~$N_{G''}(H') \subseteq N_{G''}(H) \subseteq N_G(H)$, i.e.,~$|N_{G''}(H')| \leq k$ so~$H'$ is a $k$-secluded tree in~$G''$ with~$V(H') \supseteq T$.

\begin{claim}
 For some~$v \in N_{G''}(H')$ there are~$k+2$ paths in~$G''$ between~$N_{G''}(T)$ and~$v$ that intersect only in~$v$.
\end{claim}
\begin{claimproof}
We partition the vertex set~$N_{G''}(T)$ into two sets:~$N_{H'}(T)$ and~$X := N_{G''}(T) \setminus N_{H'}(T)$. Now consider the connected components of~$H' - T$. \hui{Since~$H'$ is a tree, there are exactly~$|N_{H'}(T)| = |N_{G''}(T)| - |X|$ such components.}
  \huir{Not sure if following argument is necessary: Clearly since~$H'$ is connected, each component contains at least one vertex from~$N_{H'}(T)$, and since~$H'$ is acyclic each component also contains at most one vertex from~$N_{H'}(T)$. On the other hand, each vertex~$v \in N_{H'}(T)$ is contained in exactly one component of~$H'-T$ since~$v \in H'$ and~$v \not\in T$.}
Observe that~$N_{G''}(T) = N_G(T)$ since edges with one endpoint in~$T$ are not removed in~$G''$, so~$|N_{G''}(T)| > k(k+1)$ and~$H'-T$ has~$k(k+1) - |X|$ components.
We argue~$|X| \leq k$ by showing~$X \subseteq N_{G''}(H')$. Suppose~$v \in X$. By definition~$X \subseteq N_{G''}(T)$, so~$v \in N_{G''}(T)$. Let~$u \in T$ be a neighbor of~$v$ in~$G''$. Since~$T \subseteq V(H')$ we have~$u \in V(H')$, so either~$v \in N_{G''}(H')$ or~$v \in V(H')$. In the second case clearly~$v \in N_{H'}(T)$, but then~$v \not\in X$, a contradiction. Hence~$v \in N_{G''}(H')$, showing that~$X \subseteq N_{G''}(H')$.

Each component of~$H'-T$ contains at least one neighbor of~$N_{G''}(H')$. \hui{TODO: this is because~$G$ does not have degree-1 vertices, so the paths can always grow until they include a vertex from~$N_{G''}(H')$.}

Since there are~$k(k+1) - |X|$ components in~$H'-T$, and each has a neighbor in~$N_{G''}(H')$, there must be a vertex~$v \in N_{G''}(H')$ that is a neighbor of more than
\begin{align*}
 \frac{k(k+1) - |X|}{|N_{G''}(H')|}
 &\geq \frac{k(k+1) - |X|}{k} &&\text{Since~$H'$ is $k$-secluded in~$G''$}\\
 &= k+1 - \frac{|X|}{k}\\
 &\geq k &&\text{Since~$|X| \leq k$}
\end{align*}
components. If~$v \in N_{G''}(T)$ then there are~$k+2$ paths in~$G''$ from~$N_{G''}(T)$ to~$v$, namely at least~$k+1$ by using components adjacent to both~$v$ and~$N_{G''}(H')$, and path consisting only of the vertex~$v$ forms one more. If~$v \not\in N_{G''}(T)$ then \hui{$|X| < k$} so there are at least~$k+2$ components adjacent to both~$v$ and~$N_{G''}(H')$.
\end{claimproof}


\hui{Finally, by exhaustively removing vertices of degree at most 1 to obtain~$G'$ from~$G''$, we do not remove~$v$ or any of its neighbors, hence~$\degree_{G'}(v) \geq k+2$.}

%Suppose~$H$ is a $k$-secluded subtree of~$G$ with~$V(H) \supseteq T$, so we have~$|N_G(H)| \leq k$. Consider the graph~$G'$ obtained in the algorithm. Since~$G'$ is a subgraph of~$G$ we have that~$G' - N_G(H)$ is a subgraph of~$G - N_G(H)$, so the connected component~$H'$ of~$G'-N_G(H)$ that contains~$T$ is a subgraph of~$H$, which is the connected component of~$G - N_G(H)$ containing~$T$. So~$H'$ is a forest, and since~$T$ is a subtree of~$H'$ we have that~$H'-T$ contains~$|N_{H'}(T)| = |N_G(T)| > k(k+1)$ connected components with exactly one vertex from~$N_G(T)$. If any such component~$C$ does not contain a neighbor of~$N_G(H)$ then there is a vertex~$v \in V(C)$ with~$\degree_G(v) = 1$. Since~$v \not\in T$ this contradicts that the instance is clean, so we conclude that~$H'-T$ contains more than~$k(k+1)$ components with both a vertex from~$N_G(T)$ and a neighbor of~$N_G(H)$. Since~$|N_G(H)| \leq k$ there is a vertex~$v \in N_G(H)$ that is neighbor to more than~$k+1$ such components. It follows that~$H'$ contains at least~$k+2$ paths from~$N_G(T)$ to~$v \in N_G(H)$ that intersect only in~$v$, and hence,~$\degree_{G'}(v) \geq k+2$. \huir{This proof needs work.}

% \hui{Old proof parts:}

% Consider a maximum weight $k$-secluded subtree~$H$ of~$G$ with~$V(H) \supseteq T$.
% \begin{claim}
% For any~$v \in N_G(T)$, there is a path~$P_v = \{v,\dots,\ell_v\}$ disjoint from~$T$ such that~$V(P_v) \cap N_G(H) = \{\ell_v\}$.
% \end{claim}
% \begin{claimproof}
% Start the path at~$v$. If~$v \in N(H)$, then set~$\ell_v = v$ and we are done. Otherwise, note that since~$v \notin T$ and the instance is clean, we have~$\degree_G(v) \geq 2$ and~$v$ has exactly one neighbor in~$T$. It follows that~$v$ has at least one neighbor~$w \notin N[T]$. Add~$w$ to the path, if~$w \in N(H)$ then we are done. Since~$H$ is acyclic,~$w$ can have no neighbor in (or path to)~$T$. By adding vertices to the path this way, at some point we end up at some vertex in~$N(H)$. \jjh{some sort of inductive argument, or is handwavy good enough?} 
% \end{claimproof}

% \begin{claim}
% For any~$u,v \in N_G(T)$ with~$u \neq v$, the paths~$P_u$ and~$P_v$ are vertex-disjoint, except possibly~$\ell_u = \ell_v$. 
% \end{claim}
% \begin{claimproof}
% Since paths are disjoint from~$T$, any intersection would result in a cycle in~$H$. 
% \end{claimproof}

% By the two claims above and the fact that~$|N_G(T)| > k(k+1)$, it follows that for some vertex~$v \in N(H)$ there are at least~$k+2$ paths from~$N_G(T)$ to~$v$ that intersect only at~$v$. 
% All that is left is to argue the time needed to identify such vertex~$v$.

% \hui{Possibly incorrect linear time algorithm  to find a suitable~$v$: grow a path from each vertex in~$N_G(T)$, if you reach a degree-$\geq 3$ vertex pick an arbitrary neighbor to extend the path. If you reach a vertex taken by another path, include it but then stop extending the path. Once all paths have terminated (by meeting up with another path, finding a leaf, or a vertex with only neighbors already included in the current path), consider the graph~$G'$ obtained from~$G$ by first removing all edges that don't have an endpoint in~$T$ and are not part of a path, and then iteratively removing all leaves. Any vertex of degree~$\geq k+1$ in this graph is a suitable choice for~$v$ (maybe?).}
\end{proof}

\fi
